# Supplementary material for: Image-Space Collage and Packing with Differentiable Rendering
Source: arXiv:2406.04008 source file (2025-05-26)
Supplement: Supplementary file 1 [file 8_supp.tex]

\section{Implementation Details}

\lm{We implemented this method using PyTorch and the Adam optimizer, with learning rates of 0.02, 0.05, and 1.1 for Scale, Rotate, and Translate, respectively. All examples and experiments in this paper were conducted on a system running Ubuntu 20.04.6 LTS, equipped with an AMD EPYC 7742 64-Core Processor and eight NVIDIA A100 GPUs. Each GPU is equipped with 40GB of GDDR6 memory (with ECC).}
